# Supplementary material for: Pure nematic state in iron-based superconductor
Source: arXiv:2208.12384 source file (2023-07-26)
Supplement: Supplementary file 1 [file FeSe_nematic_SM_review2_verfinal.pdf]

Supplemental Material

# Pure nematic state in iron-based superconductor


Y. Kubota,[1] F. Nabeshima,[2] K. Nakayama,[3,4] H. Ohsumi,[1] Yoshikazu Tanaka,[1] K. Tamasaku,[1,5] T. Suzuki,[6] K. Okazaki,[6] T. Sato,[3,7] A. Maeda,[2] and M. Yabashi[1,5]

[1]*RIKEN SPring-8 Center, 1-1-1 Kouto, Sayo, Hyogo 679-5148, Japan*
[2]*Department of Basic Science, University of Tokyo, 3-8-1 Komaba, Meguro, Tokyo 153-8902, Japan*
[3]*Department of Physics, Graduate School of Science, Tohoku University, Sendai 980-8578, Japan*
[4]*Precursory Research for Embryonic Science and Technology, Japan Science and Technology Agency, Tokyo 102-0076, Japan*
[5]*Japan Synchrotron Radiation Research Institute (JASRI), 1-1-1 Kouto, Sayo, Hyogo 679-5198, Japan*
[6]*Institute for Solid State Physics, The University of Tokyo, Kashiwa, Chiba 277-8581, Japan*
[7]*Advanced Institute for Materials Research (WPI-AIMR), Tohoku University, Sendai 980-8577, Japan*


## Section 1: Characterization of the thickness of the cleaved FeSe film

As described in the experimental section in the main text, we fabricated the FeSe film with a thickness of ~300 nm for angle-resolved photoemission spectroscopy (ARPES) and cleaved it *in situ* to obtain a clean surface necessary for ARPES. The thickness of the cleaved FeSe film was determined to be ~70 nm by transmission electron microscopy (TEM)-energy dispersive x-ray spectroscopy (EDX) after the ARPES measurements [Figs. S1(a) and S1(b)]. The comparable thicknesses between the films in ARPES and x-ray diffraction (XRD) measurements would guarantee their similar properties.

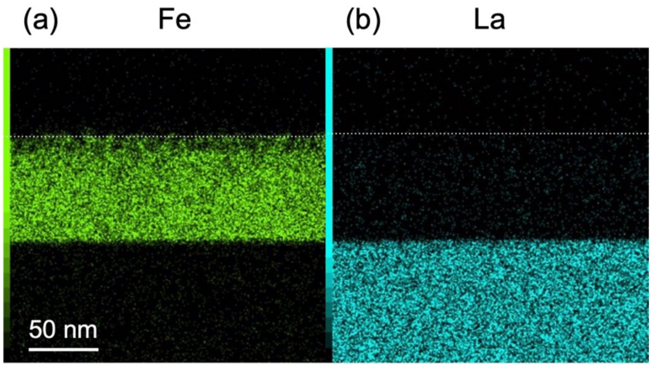


FIG. S1: (a), (b) TEM-EDX cross-sectional mapping of Fe and La, respectively, of cleaved FeSe films on LAO. These images were obtained after ARPES measurements.

## Section 2: Comparison of XRD profiles in a wide 2$\theta$ range

We have confirmed that the baselines of XRD profiles at all temperatures match in the $\Delta 2\theta$ region far from the peak position, as shown in Fig. S2 (see $0.5° < \Delta 2\theta < 1.5°$) [note that Fig. 4(b) shows a magnified view of the peak area enclosed by a dashed rectangle in Fig. S2]. Therefore, the difference in the spectral intensity at $\Delta 2\theta \sim 0.4°$ in Fig. 4(b) is not a misalignment of the baselines but an intrinsic feature originating from the gradual increase of the peak intensity at low temperatures.

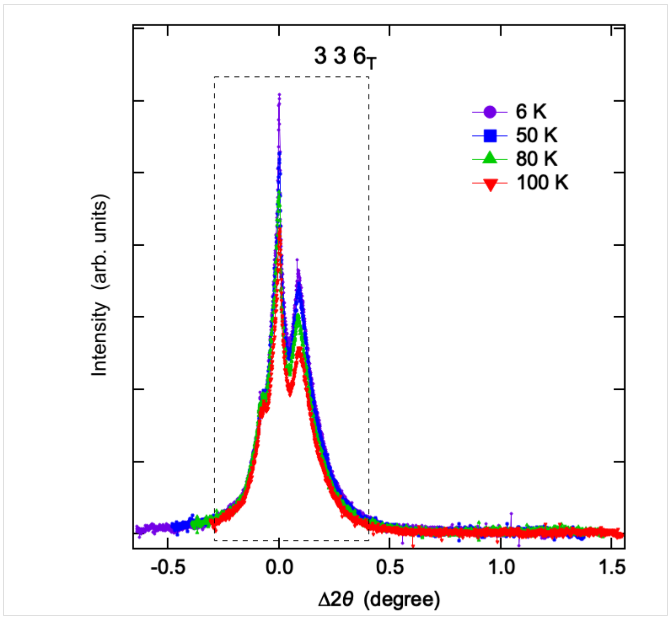


FIG. S2: Temperature dependence of the XRD profile at the $336_T$ Bragg reflection. The data are the same as Fig. 4(b) in the main text but with a larger horizontal axis range. The dashed rectangle represents the peak area shown in Fig. 4(b).

## Section 3: Temperature dependence of the peak width and area of XRD profiles

Temperature dependence of the main peak width and area were obtained by the fitting with the Lorentz function for the XRD profiles, as shown in Fig. 4(c) and Fig. S3, respectively. The peak width decreased with decreasing temperature, while the peak area increased. These behaviors indicate that the structural transition does not occur in the FeSe film.

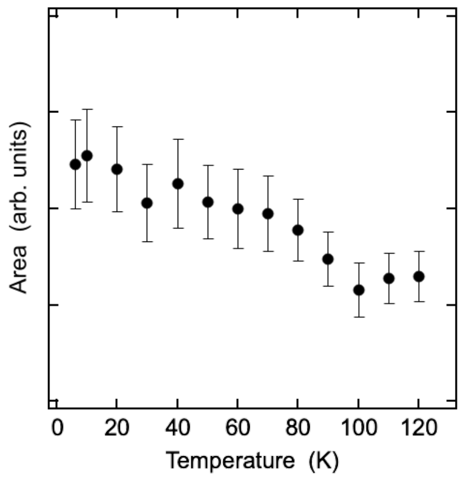


FIG. S3: Temperature dependence of the area of the main diffraction peak obtained by the fitting with the Lorentz function for the XRD profiles. The vertical bars represent error bars from the fitting.
